# Supplementary material for: On the Robustness of Tabular Foundation Models: Test-Time Attacks and In-Context Defenses
Source: arXiv:2506.02978 source file (2026-04-09)
Supplement: Supplementary file 1 [file supp_rq3_defense.tex]

% \begin{table*}[h]

% \caption{Robust accuracy and clean accuracy of different robustification strategies. (FT: finetuning, AFT: adversarial finetuning, AFT E.S.: adversarial finetuning with early stopping,  AICL: adversarial in context learning) }\label{tab:supp_rq3_results}
% \small
% %\setlength\tabcolsep{3pt}
% \begin{tabular}{llrrrrrrrrr}

% \toprule
% Dataset &  & \multicolumn{3}{c}{LCLD} & \multicolumn{3}{c}{URL} & \multicolumn{3}{c}{WIDS} \\
% \cmidrule(r){3-5} \cmidrule(r){6-8} \cmidrule(r){9-11}

%  Model & Training & Clean & CAPGD & CAA & Clean & CAPGD & CAA & Clean & CAPGD & CAA \\
% \midrule
% \multirow[c]{4}{*}{TabPFNv2} & Original & 55.2 & 13.5\tiny{$\pm 0.5$} & 7.5\tiny{$\pm 0.4$} & 97.1 & 91.2\tiny{$\pm 0.4$} & 26.5\tiny{$\pm 0.9$} & 68.2 & 63.7\tiny{$\pm 0.5$} & 28.9\tiny{$\pm 0.7$} \\
%  & AFT & 47.7 & 9.3\tiny{$\pm 0.6$} & 6.1\tiny{$\pm 0.1$} & 96.4 & 90.4\tiny{$\pm 1.0$} & 24.1\tiny{$\pm 0.5$} & 61.9 & 59.5\tiny{$\pm 0.6$} & 23.7\tiny{$\pm 0.8$} \\
%  & AFT E.S. & 55.1 & 14.6\tiny{$\pm 2.3$} & 10.8\tiny{$\pm 1.1$} & 96.4 & 92.0\tiny{$\pm 1.2$} & 27.4\tiny{$\pm 1.9$} & 68.7 & 64.3\tiny{$\pm 2.8$} & 28.0\tiny{$\pm 1.0$} \\
%  & AICL & 63.5 & 34.3\tiny{$\pm 0.9$} & 19.5\tiny{$\pm 0.3$} & 96.5 & 93.6\tiny{$\pm 0.4$} & 28.4\tiny{$\pm 0.6$} & 72.0 & 66.0\tiny{$\pm 0.5$} & 27.9\tiny{$\pm 0.8$} \\
% \cline{1-11}
% \multirow[c]{4}{*}{TabICL} & Original & 60.5 & 21.0\tiny{$\pm 0.5$} & 12.5\tiny{$\pm 0.4$} & 96.5 & 95.7\tiny{$\pm 0.2$} & 30.7\tiny{$\pm 1.1$} & 77.0 & 72.5\tiny{$\pm 0.7$} & 40.6\tiny{$\pm 1.2$} \\
%  & AFT & 60.8 & 24.4\tiny{$\pm 0.7$} & 11.9\tiny{$\pm 0.5$} & 96.3 & 94.6\tiny{$\pm 0.4$} & 26.1\tiny{$\pm 0.5$} & 58.0 & 57.3\tiny{$\pm 0.3$} & 27.6\tiny{$\pm 0.5$} \\
%  & AFT E.S. & 60.8 & 24.7\tiny{$\pm 1.0$} & 15.9\tiny{$\pm 0.5$} & 96.6 & 95.4\tiny{$\pm 0.5$} & 31.6\tiny{$\pm 1.4$} & 75.5 & 71.9\tiny{$\pm 0.2$} & 40.9\tiny{$\pm 2.0$} \\
%  & AICL & 63.0 & 47.7\tiny{$\pm 1.0$} & 37.2\tiny{$\pm 0.5$} & 96.7 & 95.1\tiny{$\pm 0.1$} & 25.1\tiny{$\pm 0.5$} & 71.2 & 70.2\tiny{$\pm 0.3$} & 49.7\tiny{$\pm 0.9$} \\
% \bottomrule
% \end{tabular}
% \end{table*}
